# Supplementary material for: UI-Voyager: A Self-Evolving GUI Agent Learning via Failed Experience
Source: arXiv:2603.24533 source file (2026-03-25)
Supplement: Supplementary file 1 [file 7_appendix.tex]

\section{Hyperparameter Details} \label{app:hyperparams}

\begin{table}[ht]
\centering
\label{tab:hyperparams_grpo}
\caption{Main Hyperparameters of GRPO}
\begin{tabular}{lll}
\toprule
Component & Hyperparameter & Value \\
\midrule
Data & Max Prompt Length & 8192 \\
Data & Max Response Length & 512 \\
Data & Train Batch Size & 256 \\
\midrule
Actor / Policy & Strategy (Parallelism) & FSDP \\
Actor / Policy & PPO Micro Batch Size/GPU & 8 \\
Actor / Policy & Learning Rate (LR) & 1e-6 \\
Actor / Policy & Gradient Clipping & 1.0 \\
Actor / Policy & Clip Ratio(low/high) & 0.2/0.28 \\
Actor / Policy & PPO Epochs & 1 \\
\midrule
Rollout \& Sampling & Sampling Temperature & 1.0 \\
Rollout \& Sampling & Max New Tokens & 512 \\
Rollout \& Sampling & Number of Samples (n) & 8 \\
Rollout \& Sampling & Max Turns & 30 \\
Rollout \& Sampling & History Length & 30 \\
% Rollout \& Sampling & Max Pixels & 5000000 \\
% Rollout \& Sampling & Min Pixels & 65536 \\
% \midrule
% Algorithm & KL Loss Coefficient & 0 \\
\bottomrule
\end{tabular}
\end{table}

\begin{table}[ht]
\centering
\label{tab:hyperparams_ppo}
\caption{Main Hyperparameters of PPO}
\begin{tabular}{lll}
\toprule
Component & Hyperparameter & Value \\
\midrule
Data & Max Prompt Length & 8192 \\
Data & Max Response Length & 512 \\
Data & Train Batch Size & 256 \\
\midrule
Actor / Policy & Strategy (Parallelism) & FSDP \\
Actor / Policy & PPO Micro Batch Size/GPU & 4 \\
Actor / Policy & Learning Rate (LR) & 1e-6 \\
Actor / Policy & Gradient Clipping & 1.0 \\
Actor / Policy & Clip Ratio & 0.2 \\
Actor / Policy & PPO Epochs & 1 \\
\midrule
Rollout \& Sampling & Sampling Temperature & 1.0 \\
Rollout \& Sampling & Max New Tokens & 512 \\
Rollout \& Sampling & Max Turns & 30 \\
% \midrule
% Algorithm & KL Loss Coefficient & 0.001 \\
% Algorithm & GAE lambda & 0.001 \\
\bottomrule
\end{tabular}
\end{table}

% \begin{table}[ht]
% \centering
% \label{tab:hyperparams_grsd}
% \caption{Main Hyperparameters of GRSD}
% \begin{tabular}{lll}
% \toprule
% Component & Hyperparameter & Value \\
% \midrule
% Data & Max Prompt Length & 16384 \\
% Data & Max Response Length & 4096 \\
% Data & Train Batch Size & 256 \\
% Data & Validation Batch Size & 256 \\
% \midrule
% Actor / Policy & Strategy (Parallelism) & FSDP \\
% Actor / Policy & PPO Micro Batch Size/GPU & 4 \\
% Actor / Policy & Learning Rate (LR) & 1e-6 \\
% Actor / Policy & Gradient Clipping & 1.0 \\
% Actor / Policy & Clip Ratio & 0.2 \\
% Actor / Policy & PPO Epochs & 1 \\
% \midrule
% Rollout \& Sampling & Sampling Temperature & 1.0 \\
% Rollout \& Sampling & Max New Tokens & 4096 \\
% Rollout \& Sampling & Number of Samples (n) & 16 \\
% Rollout \& Sampling & Max Turns & 50 \\
% Rollout \& Sampling & Max Pixels & 5000000 \\
% Rollout \& Sampling & Min Pixels & 65536 \\
% \midrule
% Algorithm & KL Loss Coefficient/ $\beta$ & 0.001 \\
% Algorithm & SPA/ $\alpha$ & 1.0 \\
% Algorithm & ADAPR/ Replay Buffer Size & 256 \\
% Algorithm & ADAPR/ $\gamma$ & 1.0 \\
% Algorithm & ADAPR/ $\kappa$ & 0.25 \\
% \bottomrule
% \end{tabular}
% \end{table}
